# Supplementary material for: Democratizing Reward Design for Personal and Representative Value-Alignment
Source: arXiv:2410.22203 source file (2024-10-29)
Supplement: Supplementary file 1 [file 8_appendix.tex]

\section{Appendix}
Demographic information table
